# Supplementary material for: The model of photoswitching in lead-halide perovskite microcrystals
Source: arXiv:2410.23823 source file (2024-10-31)
Supplement: Supplementary file 1 [file Supplementary.pdf]

# The model of photoswitching in lead-halide perovskite microcrystals: Supplementary material

Eduard A. Podshivaylov and Pavel A. Frantsuzov

Voevodsky Institute of Chemical Kinetics and Combustion SB RAS, 630090, Novosibirsk, Russia

## Supplementary material 1. Analytical solution for electron density at uniform density of deep traps

Let us consider the first equation in the system (29) in the main article, where the trap density is uniform ($N = const$) at low excitation power:

$$D_n \frac{d^2 n}{dz^2} = k_t N n - \frac{J_e}{l_e} e^{-z/l_e} \tag{1}$$

with the boundary conditions:

$$\frac{dn}{dz}(0) = \frac{dn}{dz}(L_{cr}) = 0.$$

The solution of the homogeneous part of the equation is as follows:

$$n_H(z) = C_1 \sinh\left(\frac{z}{L_D}\right) + C_2 \cosh\left(\frac{z}{L_D}\right), \tag{2}$$

where $L_D = \sqrt{D_n/k_t N}$ is the diffusion length.

The specific solution of the differential equation is:

$$n_S(z) = -\frac{J_e l_e}{D_n(1 - (l_e/L_D)^2)} \exp(-z/l_e). \tag{3}$$

Thus, the general solution is written as follows:

$$n(z) = C_1 \sinh\left(\frac{z}{L_D}\right) + C_2 \cosh\left(\frac{z}{L_D}\right) - \frac{J_e l_e}{D_n[1 - (l_e/L_D)^2]} \exp\left(-\frac{z}{l_e}\right). \tag{4}$$

The boundary conditions give the following solutions for unknown coefficients:

$$C_1 = -\frac{J_e L_D}{D_n[1 - (l_e/L_D)^2]}, \tag{5}$$

$$C_2 = \frac{J_e L_D}{D_n[1-(l_e/L_D)^2]}\left[\cosh\left(\frac{L_{cr}}{L_D}\right) - \exp\left(-\frac{L_{cr}}{l_e}\right)\right] / \sinh\left(\frac{L_{cr}}{L_D}\right). \quad (6)$$

In the limit $l_e \to 0$ the equation (1) has the following form:

$$D_n \frac{d^2 n}{dz^2} = k_t N n \quad (7)$$

with the boundary conditions:

$$-D_n \frac{dn}{dz}(0) = J_e, \; -D_n \frac{dn}{dz}(L_{cr}) = 0.$$

The solution to this equation is as follows:

$$n(z) = A_1 \sinh\left(\frac{z}{L_D}\right) + A_2 \cosh\left(\frac{z}{L_D}\right), \quad (8)$$

where the unknown coefficients are:

$$A_1 = -J_e L_D / D_n, \quad (9)$$

$$A_2 = J_e L_D / D_n \coth\left(\frac{L_{cr}}{L_D}\right). \quad (10)$$

Thus, the solution can be written as:

$$n(z) = \frac{J_e L_D}{D_n}\left[\coth\left(\frac{L_{cr}}{L_D}\right)\cosh\left(\frac{z}{L_D}\right) - \sinh\left(\frac{z}{L_D}\right)\right]. \quad (11)$$

It can be easily shown that expression (4) becomes the expression (11) at the limit $l_e \to 0$. At the rapid diffusion limit $L_D \to \infty$, the electron density (11) has the following form, which is equivalent the second equation in the system (19) in the main text:

$$n(z) = \frac{J_e}{D_n}\frac{L_D^2}{L_{cr}} = \frac{G_e}{k_t N}. \quad (12)$$

# Supplementary material 2. Analytical solution for the trap density in the rapid diffusion limit

The kinetic equation for the trap density in the rapid diffusion limit is given by Eq. (44) in the main text:

$$\frac{dN_A}{dt} = \sigma_c J_c (N_M - N_A) - \alpha G_e \frac{N_A}{N_{st} + N_A}. \quad (13)$$

Let's introduce the following variables:

$$a = \sigma_c J_c N_M N_{st},$$

$$b = \sigma_c J_c [N_M - N_{st}] - \alpha G_e,$$

$$c = -\sigma_c J_c.$$

Eq. (13) can then be written as follows:

$$\frac{dN_A}{dt} = \frac{a + bN_A + cN_A^2}{N_{st} + N_A}. \quad (14)$$

It is possible to separate variables in this equation:

$$\int_0^{N_A} \frac{N_{st} + x}{a + bx + cx^2} dx = \int_{t_{ON}}^{t} dt', \quad (15)$$

where the condition $N_A(t_{ON}) = 0$ is used. The integral on the left side depends on the sign of the discriminant of the square polynomial in the denominator:

$$D = b^2 - 4ac = b^2 + 4(\sigma_c J_c)^2 N_M N_{st}.$$

Since, the $D$ value is positive, the indefinite integral can be written as [1]:

$$\Phi(x) \equiv \int \frac{N_{st} + x}{a + bx + cx^2} dx + const, \quad (16)$$

$$\Phi(x) = \frac{1}{2c} \ln \left| a + bx + cx^2 \right| - \frac{2cN_{st} - b}{c\sqrt{D}} \tanh^{-1} \frac{2cx + b}{\sqrt{D}} + const. \quad (17)$$

Thus, from Eq. (15) we get the implicit solution:

$$\Phi(N_A(t)) - \Phi(0) = t - t_{ON}. \quad (18)$$

The trap density decreases over time until it reaches a stationary value $N_A^\infty$. The stationary density can be found from Eq.(14) by setting:

$$\frac{dN_A}{dt} = 0,$$

which is equivalent to:

$$a + bN_A^\infty + c(N_A^\infty)^2 = 0.$$

The positive solution of this equation is:

$$N_A^\infty = -\frac{b + \sqrt{D}}{2c}. \quad (19)$$

The equation of trap dynamics after the control light is switched off is:

$$\frac{dN_A}{dt} = -\alpha G_e \frac{N_A}{N_{st} + N_A}. \quad (20)$$

It's solution can be expressed in terms of Lambert's W-function:

$$N_A(t) = N_{st} W \left[ \frac{N(t_{OFF}) \exp\left(\{N(t_{OFF}) + \alpha G_e (t - t_{OFF})\}/N_{st}\right)}{N_{st}} \right]. \quad (21)$$

# Supplementary material 3. Approximate solutions for the trap and electron densities

Let us assume that the condition $l_e \to 0$ is applied. The first equation in the system (38) in the main article in this limit has the following form:

$$D_n \frac{d^2}{dz^2} n(z) = k_t N(z) n(z) \tag{22}$$

with the boundary conditions:

$$-D_n \frac{dn}{dz}(0) = J_e; \; -D_n \frac{dn}{dz}(L_{cr}) = 0. \tag{23}$$

The kinetic equation for the active trap density is given by Eq. (42) in the main article:

$$\frac{\partial N_A}{\partial t} = \sigma_c J_c e^{-z/l_c}[N_M - N_A] - \alpha k_t n N_A(z). \tag{24}$$

In the absence of the control light excitation ($J_c = 0$) the stationary solution of Eq. (24) is

$$N_A(z) = 0.$$

After switching on the control light the trap density grows and PL intensity decays. Unfortunately, an analytical solution of the Eqs. (22-24) in general case is not possible. Let us consider approximate solutions on some limiting cases.

## Moving boundary approximation

If the following conditions are met:

$$l_c \gg L_{cr}, \quad \sigma_c J_c \gg \alpha k_t n$$

the Eq. (24) can be rewritten as:

$$\frac{\partial}{\partial t} N_A(z,t) = \sigma_c J_c (N_M - N_A(Z,t)). \tag{25}$$

The solution of this equation has the following form:

$$N_A(z,t) = N_M (1 - \exp(-\sigma_c J_c (t - t_{ON}))).$$

Thus, the PL intensity decays with the falling rate:

$$\Gamma_F \approx \sigma_c J_c.$$

After the time period $\Gamma_F^{-1}$ the density of traps reaches the uniform value:

$$N_A(z) = N_M.$$

After the control light is switched off, the trap density begins to decay in the area close to the beginning of the crystal. The trap density can be described by the following approximation.

$$N_A(z,t) = 0, \text{ for } z < Z(t),$$

where $Z(t)$ is the coordinate of the boundary between areas with low and high trap densities. At $z > Z(t)$ the density $N_A$ rapidly increases and after a short intermediate zone reaches $N_M$. The electron density rapidly decays at $z > Z(t)$, so we can apply a boundary condition:

$$n(Z(t)) = 0$$

. The solution of Eq.(22) is:

$$n(z) = n_0 \sinh\left(\frac{Z(t) - z}{L_D}\right) \text{ for } z < Z(t),$$

where

$$L_D = \sqrt{\frac{D_n}{k_t N_{st}}}.$$

From the boundary condition (23) we get:

$$n_0 = \frac{J_e}{\sqrt{k_t N_{st} D_n}} \cosh^{-1}\left(\frac{Z(t)}{L_D}\right). \tag{26}$$

Thus, the diffusion flux through the border is:

$$J(Z(t)) = -D_n \frac{dn}{dz}(Z(t)) = J_e \cosh^{-1}\left(\frac{Z(t)}{L_D}\right),$$

From Eq.(24) it follows:

$$\frac{d}{dt} \int_{Z(t)}^{L_{cr}} N_A(z,t)\, dz = -\alpha k_t \int_{Z(t)}^{L_{cr}} N_A(z,t) n(z)\, dz \approx \alpha \int_{Z(t)}^{L_{cr}} N(z,t) n(z)\, dz. \tag{27}$$

Applying Eq.(22) we have:

$$\frac{d}{dt} \int_{Z(t)}^{L_{cr}} N_A(z,t)\, dz \approx -\alpha J(Z(t)). \tag{28}$$

The decay of the total number of the traps follows the movement of the boundary. Finally we have the following equation:

$$\frac{d}{dt} Z(t) \approx \alpha \frac{J_e}{N_M} \cosh^{-1}\left(\frac{Z(t)}{L_D}\right). \tag{29}$$

We can estimate the characteristic time scale for the boundary to reach the other side of the crystal:

$$\tau \approx \frac{L_{cr} N_M}{\alpha J_e}, \tag{30}$$

which corresponds to the following rising rate:

$$\Gamma_R \approx \frac{\alpha J_e}{L_{cr} N_M}. \tag{31}$$

It can be seen that the rate is proportional to the intensity of the excitation light and inversely proportional to the number of traps initially created, which explains the dependence of the rising rate on the switching efficiency in the photoswitching curve.

Numerical simulations of Eqs. (22-24) are consistent with the moving boundary approximation. As seen in Fig. S1 the trap distribution shows a boundary between areas with low and high trap densities moving from one edge of the crystal to the other.

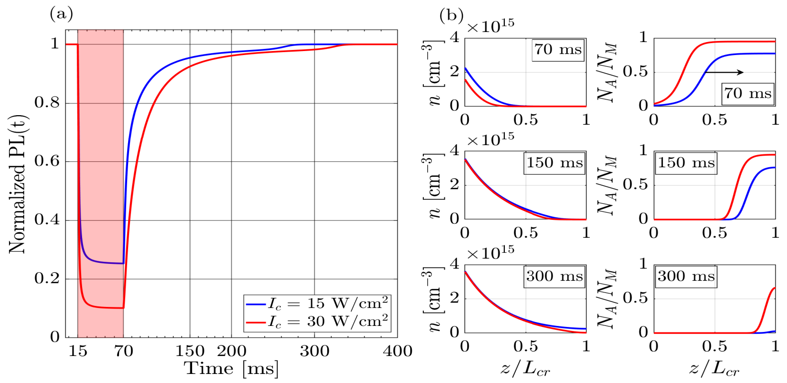


Figure S1: (a) The time dependence of PL intensity for two values of the control light power. (b) The electron density and trap density profiles at different time points. The excitation light intensity is 5 W/cm$^2$.

The parameters chosen for this approximation are as follows: $N_{st} = 5 \times 10^{15}$cm$^{-3}$, $\lambda_e = 450$ nm, $\lambda_c = 600$ nm, $N_M = 2.5 \times 10^{17}$cm$^{-3}$, $\alpha = 3 \times 10^{-4}$, $\sigma_c = 6 \times 10^{-19}$cm$^2$, $k_t = 2 \times 10^{-9}$cm$^3$s$^{-1}$, $k_n = 2 \times 10^{-5}$cm$^3$s$^{-1}$, $L_{cr} = 10$ $\mu$m, $D_n = 1$ cm$^2$s$^{-1}$, $D_p = 1$ cm$^2$s$^{-1}$.

## Wentzel-Kramers-Brullien approximation

In the case when the condition $l_c \gg L_{cr}$ does not apply, the trap density after the switching off the control light is not uniform. Thus, the moving boundary approximation cannot be applied to solve Eq.(22). Since the following condition applies

$$\frac{k_t N(z)}{D_n} L_{cr}^2 \gg 1,$$

it is possible to use the Wentzel-Kramers-Brullien approximation:

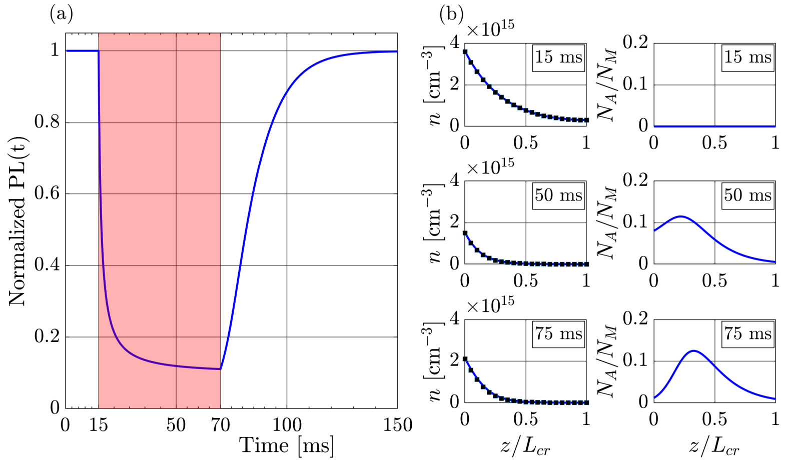


Figure S2: (a) The time dependence of PL intensity. (b) Profiles of the electron density (curves - numerical solution of the Eq.(22), squares - WKB approximation) and trap density at different time points. The excitation light intensity is 5 W/cm$^2$, control light intensity is 15 W/cm$^2$.

$$n(z) = \sum_{+,-} \frac{C_\pm}{g^{1/4}(z)} \exp\left[\pm \int_0^z \sqrt{g(z)}dz\right], \tag{32}$$

where $g(z) = [1+N_A/N_{st}]/L_D^2$, $L_D = \sqrt{D_n/k_t N_{st}}$, and the unknown coefficients equations are:

$$\sum_{+,-} \frac{C_\pm}{g^{1/4}(0)} \left(-\frac{g'(0)}{4g(0)} \pm \sqrt{g(0)}\right) = -J_e/D_n, \tag{33}$$

$$\sum_{+,-} \frac{C_\pm}{g^{1/4}(L_{cr})} \left(-\frac{g'(L_{cr})}{4g(L_{cr})} \pm \sqrt{g(L_{cr})}\right) \exp\left[\pm \int_0^{L_{cr}} \sqrt{g(z)}dz\right] = 0. \tag{34}$$

In order to check the resulting approximation, we carried out two numerical tests. Fig. S2 shows a comparison of the numerical solution of the basic equation and the WKB method solution. It can be seen that in the three most interesting cases, the solutions are practically identical. There is a slight difference due to the fact that the derivative included in the expression for the coefficients was searched numerically, since there is no analytical expression for it from the equation for the dynamics of traps.

Fig. S3 shows the same comparison, but the intensity of the control light is significantly increased. Indeed, it is clear that the WKB method differs significantly from the numerical solution, which cannot be explained by calculation

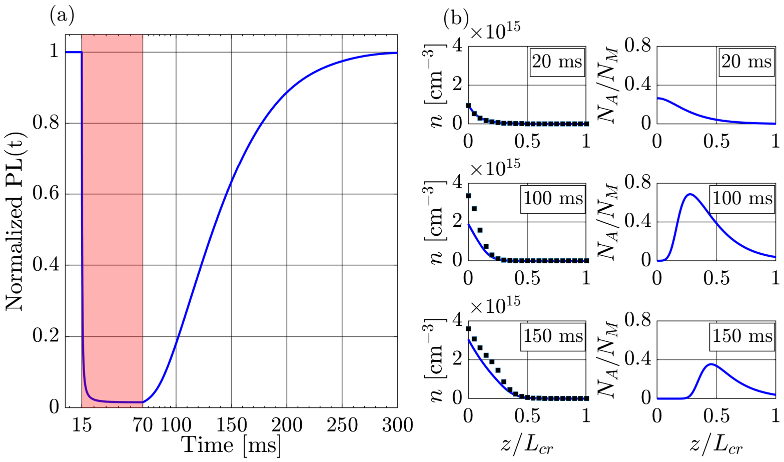


Figure S3: (a) The time dependence of PL intensity. (b) Profiles of the electron density (curves - numerical solution of the Eq.(22), squares - WKB approximation) and trap density at different time points. The excitation light intensity is 5 W/cm$^2$, control light intensity is 60 W/cm$^2$.

errors. This discrepancy is due to a violation of the conditions of applicability of the Wentzel-Kramers-Brillouin method. This condition can be written as follows:

$$|g'| \ll 2g^{3/2}. \tag{35}$$

The case of the high intensity control light roughly corresponds to the case from the previous subsection. The density of the created traps is a large value, but it has a sharp difference in the area between the destroyed traps and the filled layers. Such a sharp drop in density makes the desired derivative large, which violates the condition of applicability of the WKB method. Thus, it becomes clear that although the Wentzel-Kramers-Brillouin method can be used at low control light intensities, it is not suitable in the general case.

The parameters chosen for these calculations are as follows: $N_{st} = 5 \times 10^{15}$cm$^{-3}$, $\lambda_e = 450$ nm, $\lambda_c = 600$ nm, $N_M = 2.5 \times 10^{17}$cm$^{-3}$, $\alpha = 10^{-4}$, $\sigma_c = 6 \times 10^{-19}$cm$^2$, $k_t = 2 \times 10^{-9}$cm$^3$s$^{-1}$, $k_n = 2 \times 10^{-5}$cm$^3$s$^{-1}$, $L_{cr} = 10$ $\mu$m, $l_c = 2$ $\mu$m, $D_n = 1$ cm$^2$s$^{-1}$, $D_p = 1$ cm$^2$s$^{-1}$.

## Supplementary material 4. Estimation of the $\tilde{p}$ value

Integrating Eq.(22) over the entire definition domain, we get the following relation:

$$\frac{1}{L_{cr}} \int_0^{L_{cr}} k_t N(z) n(z) dz = \frac{J_e}{L_{cr}} = G_e. \tag{36}$$

Let's introduce the average carrier density as follows:

$$\overline{n} = \frac{1}{L_{cr}} \int_0^{L_{cr}} n(z)\, dz. \tag{37}$$

From Eq.(36) it follows that:

$$\overline{n} < \overline{n}_{max} \equiv \frac{G_e}{k_t N_{st}}. \tag{38}$$

According to Eq.(30) in the main article $n(z)$ and $p(z)$ are connected:

$$p(z) = \frac{D_n}{D_p} n(z) + \tilde{p}.$$

The value of the parameter $\tilde{p}$ can be found using the charge conservation law Eq.(34) of the main article, which can be rewritten as:

$$\tilde{p} L_{cr} = (1-x)\overline{n} L_{cr} + \frac{k_t}{k_n} \int_0^{L_{cr}} \frac{N(z)n(z)}{xn(z) + \tilde{p}}\, dz, \tag{39}$$

where $x = D_n/D_p$. We obtain a rough estimate for the value of $\tilde{p}$ by replacing the density in the denominator of an integrand with the maximum average density and using the relation (36):

$$\tilde{p} > (1-x)\overline{n} + \frac{k_t/k_n L_{cr}}{(x\overline{n}_{\max} + \tilde{p})} \int_0^{L_{cr}} N(z)n(z)\, dz = (1-x)\overline{n} + \frac{G_e}{k_n(x\overline{n}_{\max} + \tilde{p})}. \tag{40}$$

If we consider the case when $x \leq 1$, then the estimation can be further simplified:

$$\tilde{p} > (1-x)\overline{n} + \frac{G_e}{k_n} \frac{1}{x\overline{n}_{\max} + \tilde{p}} > \frac{G_e}{k_n} \frac{1}{\overline{n}_{\max} + \tilde{p}}. \tag{41}$$

In this case, we get the following inequality:

$$\tilde{p}(\tilde{p} + \overline{n}_{\max}) - \frac{G_e}{k_n} > 0. \tag{42}$$

The only positive bound is as follows:

$$\tilde{p} > \frac{1}{2}\left[\sqrt{\overline{n}_{\max}^2 + \frac{4G_e}{k_n}} - \overline{n}_{\max}\right]. \tag{43}$$

On the other hand, the estimation with $n(z) = 0$ in the denominator of (39) leads to:

$$\tilde{p} < \frac{1}{2}\left[(1-x)\overline{n} + \sqrt{(1-x)^2\overline{n}^2 + \frac{4G_e}{k_n}}\right]. \tag{44}$$

In the case of $\overline{n} \gg \sqrt{G_e/k_n}$ (ABC regime) the following is true:

$$0 < \tilde{p} < (1-x)\overline{n}. \tag{45}$$

If $x \approx 1$,*i.e.* the diffusion coefficients are close, the $\tilde{p}$ tends to 0, so that $n(z) \approx p(z)$. In the opposite case (SRH regime) the next condition is true:

$$\sqrt{\frac{G_e}{k_n}} < \tilde{p} < \sqrt{\frac{G_e}{k_n}}, \tag{46}$$

so $p(z) \approx \tilde{p} = \sqrt{\frac{G_e}{k_n}} \gg \overline{n}_{\max}$.

# Supplementary material 5. Details on numerical calculation

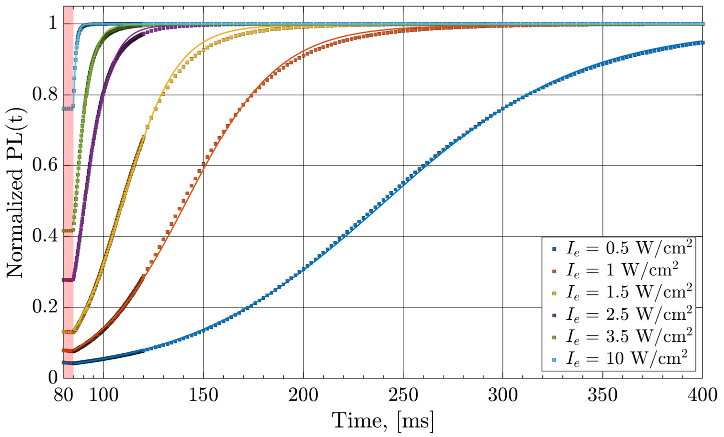


Figure S4: Simulated PL rising curves for different excitation light intensities (colored squares), and their fit using a logistic function (colored lines). Control light intensity is 15 W/cm$^2$.

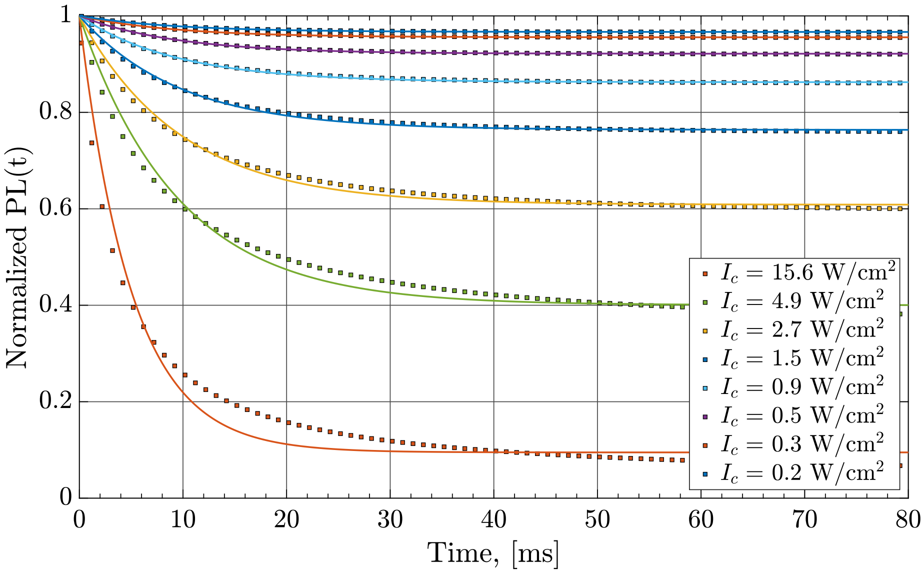


Figure S5: Simulated PL falling curves for different control light intensities (colored squares), and their fit using an exponential decay function (colored lines). Excitation light intensity is 1 W/cm$^2$.

The electron density equation was solved for each time step using the implicit first-order method for the boundary value problem with a step size of $L_{cr}/200$. The traps dynamics was tested on three different integration schemes: the first-order Euler scheme, the second-order Euler scheme with corrections, and the fourth-order Runge-Kutta scheme. We have found the step sizes consistent for all 3 schemes, however, the most time-efficient scheme with an acceptable resolution was the Euler scheme with corrections. The time step depend on parameters and therefore differs for different calcultions. The solution for charge conservation equation with the constant $\tilde{p}$ was found using the standard MATLAB fzero function. All spatial integrals were calculated using the left-rectangular method.

The falling rate was determined as the characteristic fit time of the model curve by exponential decay using the least squares method with fminsearch MATLAB function. The rising rate was determined as the characteristic fit time of the model curve by logistic growth curve using the least squares method. Here we present images corresponding to calculations for rising and falling rates. In the case of rising, the logistic curve is almost always a good fit, as shown in Fig. S4. However, in the case of the falling curve, deviations from the ideal exponential decay are observed in Fig. S5 at control light intensities, that correspond to switching efficiencies larger than 0.5. The parameters selected for these calculations match the model parameters in the case of a short extinction length of the excitation light from the main text.

Fig. S6 contains the falling rate dependence on control light intensity with different excitation light intensities. It can be seen that the saturation on low control light intensities is caused by the presence of the excitation light. The parameters match the parameters in Fig. S4-S5, but $\sigma_c = 6 \times 10^{-19}$ cm$^{-2}$.

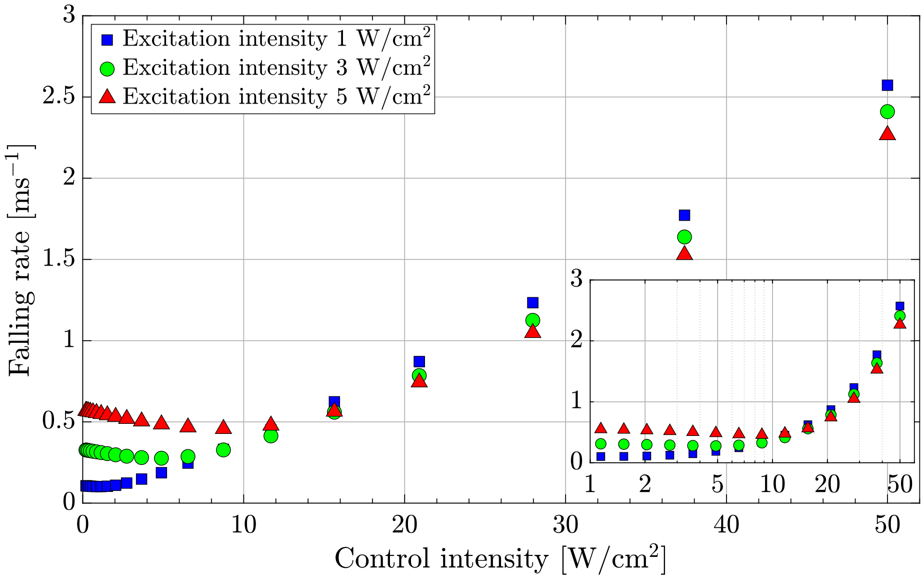


Figure S6: The control light intensity dependence of the falling rate on control light at different excitation light intensities. The insert: the same dependence but in logarithmic scale on control light intensity.

# Supplementary material 6. Numerical simulations for different trap annihilation processes

In order to check applicability of the trap annihilation mechanisms suggested in the Discussion section in the main article, we carried out numerical simulations of the PL time dependence. Figs. S7-S11 show PL time dependencies for various control light intensities found for various annihilation mechanisms. It can be seen that the photoswitching curve does not reproduce the properties observed in experiment, and moreover, the processes considered do not allow the luminescence to completely recover during the photoswitching process in many cases. This occurred because, with the selected parameters for carrier diffusion, carriers did not reach the second face of the crystal, and traps had not been completely annihilated during the process. Thus, the annihilation processes considered are not valid for the description of the traps dynamics. The specific rate constants of the considered process are indicated in the caption of the corresponding figures.

The parameters of the model are as follows: $N_{st} = 5 \times 10^{15}$cm$^{-3}$, $\lambda_e = 450$ nm, $\lambda_c = 600$ nm, $N_M = 2.5{\times}10^{17}$cm$^{-3}$, $\sigma_c = 6{\times}10^{-19}$cm$^2$, $k_t = 2{\times}10^{-9}$cm$^3$s$^{-1}$, $k_n = 2 \times 10^{-5}$cm$^3$s$^{-1}$, $L_{cr} = 10$ $\mu$m, $l_c = 2$ $\mu$m, $D_n = 1$ cm$^2$s$^{-1}$, $D_p = 1$ cm$^2$s$^{-1}$, $I_e = 1$ W/cm$^2$.

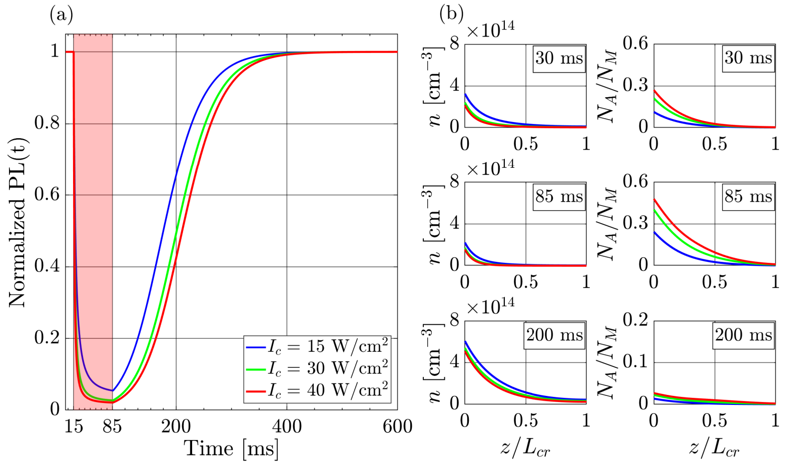


Figure S7: (a) PL intensity as a function of time at different control light intensities. (b) Profiles of the electron density and trap density at different times. $R_A = k_s n_t^{(A)}$, $k_s = 250$ ms$^{-1}$.

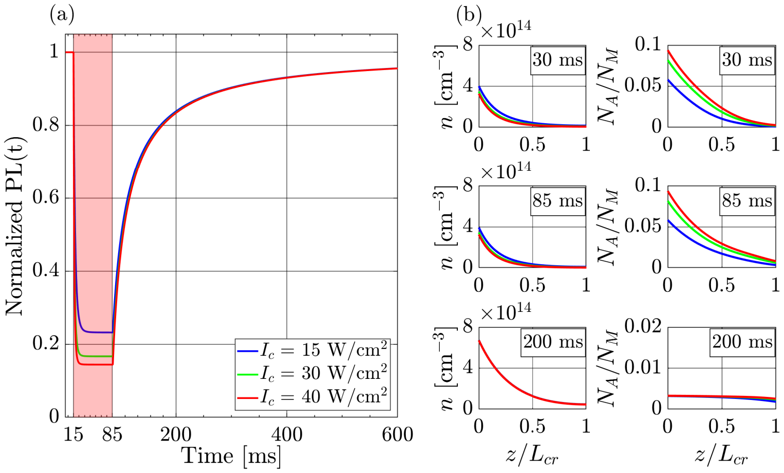


Figure S8: (a) PL intensity as a function of time at different control light intensities. (b) Profiles of the electron density and trap density at different times. $R_A = Kn_t^{(A)}n_t^{(A)}$, $K = 10^{-9}$ cm$^3$ms$^{-1}$.

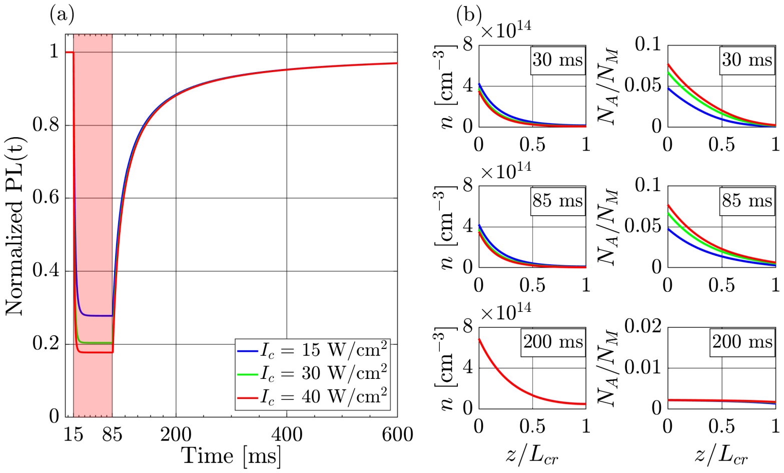


Figure S9: (a) PL intensity as a function of time at different control light intensities. (b) Profiles of the electron density and trap density at different times. $R_A = Kn_t^{(A)}N_A$, $K = 1.5 \times 10^{-13}$ cm$^3$ms$^{-1}$.

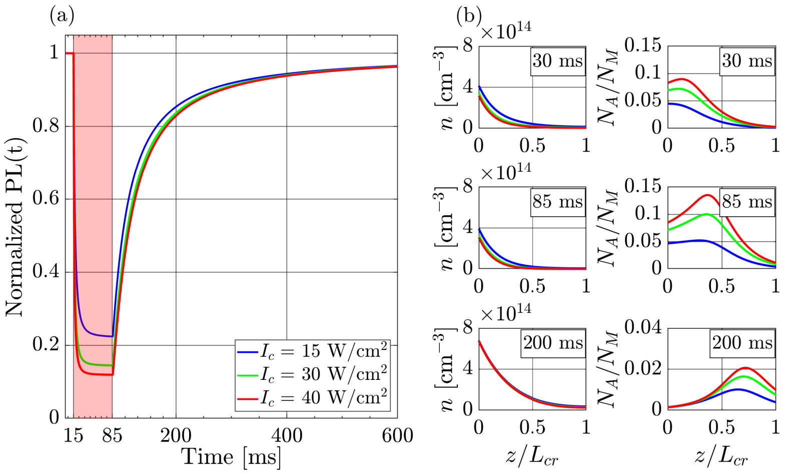


Figure S10: (a) PL intensity as a function of time at different control light intensities. (b) Profiles of the electron density and trap density at different times. $R_A = KnN_A^2$, $K = 4 \times 10^{-32}$ cm$^6$ms$^{-1}$.

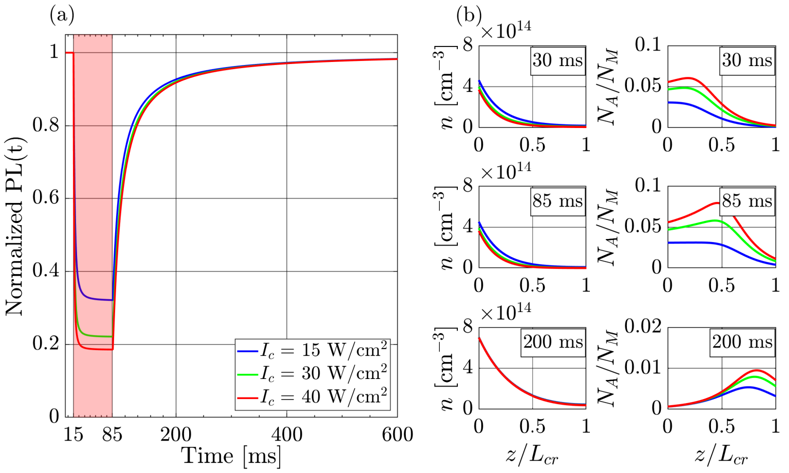


Figure S11: (a) PL intensity as a function of time at different control light intensities. (b) Profiles of the electron density and trap density at different times. $R_A = Knn_t^{(A)}N_A$, $K$ =$8 \times 10^{-28}$ cm$^6$ms$^{-1}$.

## References

[1] A.P. Prudnikov, I.U.A. Brychkov, and O.I. Marichev. *Integrals and Series: Elementary functions.* Integrals and Series. Gordon and Breach Science Publishers, 1986.
